# Supplementary material for: Short-range expansion for the quantum many-body problem
Source: arXiv:2307.05910 source file (2023-07-12)
Supplement: Supplementary file 1 [file Supplementary_short_range_expansion.pdf]

LA-UR-23-27155

# Short-range expansion for the quantum many-body problem - Supplemental Material

Ronen Weiss,[1,*] Diego Lonardoni,[1,†] and Stefano Gandolfi[1]
[1] Theoretical Division, Los Alamos National Laboratory, Los Alamos, New Mexico 87545, USA
(Dated: July 11, 2023)

## I. DEFINITION AND PROPERTIES OF CONTACTS

In this section we provide more details regarding the definition of the contacts and their properties. We consider the case of no coupled channels. In the manuscript, the following expansion of the many-body wave function was derived

$$\Psi(\boldsymbol{r}_1, ..., \boldsymbol{r}_A) = \sum_{n=0}^{\infty} \sum_{\alpha} \varphi_{\alpha}^{(n)}(\boldsymbol{r}_{12}) A_{\alpha}^{(n)}(\boldsymbol{R}_{12}, \boldsymbol{r}_3, ..., \boldsymbol{r}_A) \tag{1}$$

where

$$\varphi_{\alpha}^{(n)}(\boldsymbol{r}_{12}) = \frac{d^n}{dE^n} \varphi_{\alpha}^{E=0}(\boldsymbol{r}_{12}) \tag{2}$$

is the $n$-th energy derivative of the two-body function evaluated at $E = 0$ (for $n = 0$ this is the zero-energy two-body wave function without any derivatives).

We consider a many-body state $\Psi$ with angular momentum quantum numbers $J, M$, which is fully anti-symmetric. We can define the following contact parameters

$$C_{\alpha\beta}^{mn}(JM) = \frac{A(A-1)}{2} \langle A_{\alpha}^{(m)} | A_{\beta}^{(n)} \rangle. \tag{3}$$

Notice that $\left(C_{\alpha\beta}^{mn}(JM)\right)^* = C_{\beta\alpha}^{nm}(JM)$. In nuclear systems, the pair quantum numbers are generally given by $\alpha = (\pi_\alpha, s_\alpha, j_\alpha, m_\alpha, t_\alpha, t_{z,\alpha})$, i.e. the parity, spin, angular momentum and isospin. For $m = n = 0$, this definition coincides with the previous definition of the $M$-dependent contacts in the Generalized Contact Formalism (GCF) [1]. As for the latter, $C_{\alpha\beta}^{mn}(JM) = 0$ if $m_\alpha \neq m_\beta$, or if $\pi_\alpha \neq \pi_\beta$, or if $t_{z,\alpha} \neq t_{z,\beta}$. It is also useful to define the M-averaged contacts

$$C_{\alpha\beta}^{mn} = \frac{1}{2J+1} \sum_{M} C_{\alpha\beta}^{mn}(JM). \tag{4}$$

They are diagonal in $j$ (in addition to $m$, $\pi$ and $t_z$), and independent of $m_\alpha$ and $m_\beta$. We also note that $\sum_{m_\alpha} C_{\alpha\alpha}^{mn}(JM)$ is independent of $M$.

Finally, we can also define the following contact parameters

$$C_{\alpha}^{mn} = S_{mn} \sum_{m_\alpha} \left(C_{\alpha\alpha}^{mn} + C_{\alpha\alpha}^{nm}\right). \tag{5}$$

Notice the notation with a single $\alpha$ subscript and the sum over $m_\alpha$ included in the definition. We can equivalently use the non-M-averaged contacts in the definition of $C_\alpha^{mn}$ because after the sum over $m_\alpha$ the M-dependence disappears. This is the contact definition used in the manuscript to describe the two-body density and one-body momentum distribution (see more details in Sec. II). These contacts are real because $(C_{\alpha\alpha}^{mn})^* = C_{\alpha\alpha}^{nm}$. Also, $C_\alpha^{mn} = C_\alpha^{nm}$.

---

* ronenw@lanl.gov
† Present affiliation: XCP-2: Eulerian Codes Group, Los Alamos National Laboratory, Los Alamos, New Mexico 87545, USA

## II. TWO-BODY DENSITY EXPANSION

In this section we present the derivation of the expansion for the two-body density. As above, we consider a many-body state $\Psi$ with angular momentum quantum numbers $J, M$, which is fully anti-symmetric. The two-body density as a function of the *vector* $\boldsymbol{r}$ is given by

$$\rho_2^{JM}(\boldsymbol{r}) = \sum_{m,n}\sum_{\alpha,\beta}\varphi_\alpha^{(m)\dagger}(\boldsymbol{r})\varphi_\beta^{(n)}(\boldsymbol{r})C_{\alpha\beta}^{mn}(JM). \tag{6}$$

We used here the expansion given in Eq. (1) and the definition of the contacts from Eq. (3). The two-body density is normalized to the number of pairs, i.e. $\int d^3r\rho_2^{JM}(\boldsymbol{r}) = A(A-1)/2$. We can look on the M-averaged two-body density $\rho_2(\boldsymbol{r}) \equiv (2J+1)^{-1}\sum_M \rho_2^{JM}(\boldsymbol{r})$. This will involve the M-averaged contacts of Eq. (4). They are diagonal in $j$, $m$, $t_z$ and $\pi$, and the two-body part $\varphi_\alpha^{(m)\dagger}(\boldsymbol{r})\varphi_\beta^{(n)}(\boldsymbol{r})$ ensures also that $s_\alpha$ must be equal to $s_\beta$ and the same for $t_\alpha = t_\beta$. Therefore, only $\alpha = \beta$ contributes, and we get

$$\rho_2(\boldsymbol{r}) = \sum_{m,n}\sum_{\alpha}\varphi_\alpha^{(m)\dagger}(\boldsymbol{r})\varphi_\alpha^{(n)}(\boldsymbol{r})C_{\alpha\alpha}^{mn}. \tag{7}$$

We can now include an integral over the angles, and define $\rho_2(r) \equiv \int d\Omega_r \rho_2(\boldsymbol{r})$ (notice that we could also perform the angle integration on $\rho_2^{JM}(\boldsymbol{r})$, because after integrating over the angles the M-dependence disappears). To perform the angle integration explicitly, we can write the two-body functions in the following way

$$\varphi_\alpha^{E=0}(\boldsymbol{r}) = \left[\phi_{\{\ell_\alpha,s_\alpha,j_\alpha,t_\alpha\}}^{E=0}(r)Y_{\ell_\alpha}(\hat{\boldsymbol{r}})\otimes\chi_{s_\alpha}\right]^{j_\alpha m_\alpha}\eta_{t_\alpha,t_{z,\alpha}}, \tag{8}$$

where $\chi_{s\mu}$ is the spin function, $\eta_{t,t_z}$ is the isospin function, and $Y_{\ell m}$ are the spherical harmonics. Therefore,

$$\varphi_\alpha^{(n)}(\boldsymbol{r}) = \left[\phi_{\{\ell_\alpha,s_\alpha,j_\alpha,t_\alpha\}}^{(n)}(r)Y_{\ell_\alpha}(\hat{\boldsymbol{r}})\otimes\chi_{s_\alpha}\right]^{j_\alpha m_\alpha}\eta_{t_\alpha,t_{z,\alpha}}, \tag{9}$$

where $\phi_{\{\ell_\alpha,s_\alpha,j_\alpha,t_\alpha\}}^{(n)}(r) = \frac{d^n}{dE^n}\phi_{\{\ell_\alpha,s_\alpha,j_\alpha,t_\alpha\}}^{E=0}(r)$. The angle integration of the two-body functions is then given by

$$\begin{aligned}\int d\Omega_r\varphi_\alpha^{(m)\dagger}(\boldsymbol{r})\varphi_\alpha^{(n)}(\boldsymbol{r}) &= \int d\Omega_r\left[\phi_{\{\ell_\alpha,s_\alpha,j_\alpha,t_\alpha\}}^{(m)}(r)Y_{\ell_\alpha}(\hat{\boldsymbol{r}})\otimes\chi_{s_\alpha}\right]^{j_\alpha m_\alpha\dagger}\left[\phi_{\{\ell_\alpha,s_\alpha,j_\alpha,t_\alpha\}}^{(n)}(r)Y_{\ell_\alpha}(\hat{\boldsymbol{r}})\otimes\chi_{s_\alpha}\right]^{j_\alpha m_\alpha}\\
&= \phi_{\{\ell_\alpha,s_\alpha,j_\alpha,t_\alpha\}}^{(m)*}(r)\phi_{\{\ell_\alpha,s_\alpha,j_\alpha,t_\alpha\}}^{(n)}(r)\int d\Omega_r\sum_{\mu,\mu',m,m'}\langle j_\alpha m_\alpha|\ell m s_\alpha\mu\rangle Y_{\ell_\alpha m}^*(\hat{\boldsymbol{r}})\chi_{s_\alpha\mu}^\dagger\langle\ell m' s_\alpha\mu'|j_\alpha m_\alpha\rangle Y_{\ell_\alpha m'}(\hat{\boldsymbol{r}})\chi_{s_\alpha\mu'}\\
&= \phi_{\{\ell_\alpha,s_\alpha,j_\alpha,t_\alpha\}}^{(m)*}(r)\phi_{\{\ell_\alpha,s_\alpha,j_\alpha,t_\alpha\}}^{(n)}(r)\sum_{\mu,m}\langle j_\alpha m_\alpha|\ell m s_\alpha\mu\rangle\langle\ell m s_\alpha\mu|j_\alpha m_\alpha\rangle\\
&= \phi_{\{\ell_\alpha,s_\alpha,j_\alpha,t_\alpha\}}^{(m)*}(r)\phi_{\{\ell_\alpha,s_\alpha,j_\alpha,t_\alpha\}}^{(n)}(r).\end{aligned} \tag{10}$$

We can choose the radial functions to be real and in this case we get

$$\int d\Omega_r\varphi_\alpha^{(m)\dagger}(\boldsymbol{r})\varphi_\alpha^{(n)}(\boldsymbol{r}) = \phi_{\{\ell_\alpha,s_\alpha,j_\alpha,t_\alpha\}}^{(m)}(r)\phi_{\{\ell_\alpha,s_\alpha,j_\alpha,t_\alpha\}}^{(n)}(r) = \int d\Omega_r\varphi_\alpha^{(n)\dagger}(\boldsymbol{r})\varphi_\alpha^{(m)}(\boldsymbol{r}). \tag{11}$$

Finally, we obtain the following expression for the angle-integrated density $\rho_2(r)$:

$$\begin{aligned}\rho_2(r) &= \sum_{m,n}\sum_{\ell_\alpha,s_\alpha,j_\alpha,t_\alpha}\left(\sum_{m_\alpha,t_{z,\alpha}}C_{\alpha\alpha}^{mn}\right)\phi_{\{\ell_\alpha,s_\alpha,j_\alpha,t_\alpha\}}^{(m)}(r)\phi_{\{\ell_\alpha,s_\alpha,j_\alpha,t_\alpha\}}^{(n)}(r)\\
&= \sum_{m\le n}S_{mn}\sum_{\ell_\alpha,s_\alpha,j_\alpha,t_\alpha}\left(\sum_{m_\alpha,t_{z,\alpha}}(C_{\alpha\alpha}^{mn}+C_{\alpha\alpha}^{nm})\right)\phi_{\{\ell_\alpha,s_\alpha,j_\alpha,t_\alpha\}}^{(m)}(r)\phi_{\{\ell_\alpha,s_\alpha,j_\alpha,t_\alpha\}}^{(n)}(r),\end{aligned} \tag{12}$$

where $S_{mn} = 1$ if $m \neq n$ and $S_{mn} = 1/2$ if $m = n$. Notice that we moved from a double sum over $m$ and $n$ to a double sum over $m \le n$. For $m = n$ we have double counting of the contacts and this is the reason for introducing the factor $S_{mn}$. With the definition of the contacts in Eq. (5), we obtain

$$\rho_2(r) = \sum_{m\le n}\sum_{\ell_\alpha,s_\alpha,j_\alpha,t_\alpha}\left(\sum_{t_{z,\alpha}}C_\alpha^{mn}\right)\phi_{\{\ell_\alpha,s_\alpha,j_\alpha,t_\alpha\}}^{(m)}(r)\phi_{\{\ell_\alpha,s_\alpha,j_\alpha,t_\alpha\}}^{(n)}(r). \tag{13}$$

## III. POWER COUNTING OF THE EXPANSION

To understand the power counting of the short-range expansion presented in the manuscript, we analyze in this section the two-body Schrödinger equation with a central potential $V(r)$. If $\phi^E(r)$ is the radial part of a two-body eigenstate with energy $E$, then $u^E(r) \equiv r\phi^E(r)$ obeys the equation

$$-\frac{\hbar^2}{2\mu}u^{E\prime\prime}(r) + \left[V(r) + \frac{\hbar^2}{2\mu}\frac{\ell(\ell+1)}{r^2}\right]u^E(r) = Eu^E(r), \tag{14}$$

where $\ell$ is the orbital angular momentum. Since we are interested in the short-range behavior of $u^E(r)$, we will consider the following expansion

$$u^E(r) = \sum_{i=1}^{\infty} a_i r^i. \tag{15}$$

Notice that the sum starts with $i = 1$ (and not $i = 0$) to keep $\phi^E(r)$ finite at $r = 0$. We also assume that the potential can be similarly expanded (at least for some neighborhood of $r = 0$)

$$V(r) = \sum_{i=0}^{\infty} V_i r^i. \tag{16}$$

To find the leading-order term of $u^E(r)$ at short distances, we substitute $u^E(r) \sim r^n$ $(n \geq 1)$ into Eq. (14):

$$-\frac{\hbar^2}{2\mu}n(n-1)r^{n-2} + V(r)r^n + \frac{\hbar^2}{2\mu}\ell(\ell+1)r^{n-2} = Er^n. \tag{17}$$

The terms $Er^n$ and $V(r)r^n$ are negligible for $r \to 0$, and so we obtain

$$n(n-1) = \ell(\ell+1). \tag{18}$$

Therefore, $n = \ell + 1$ or $n = -\ell$. Since $n \geq 1$, only

$$n = \ell + 1 \tag{19}$$

is possible. This means that $a_i = 0$ for all $i \leq \ell$, and $a_{\ell+1}$ is the first non-zero coefficient in the expansion of $u^E(r)$. We can choose $a_{\ell+1} = 1$. This gives us the behavior of two-body eigenstates at very short distances. Notice that this behavior does not depend on the energy.

To study the behavior of the energy derivatives of the two-body functions, we need to continue to the next term in the expansion. For this purpose we substitute $u^E(r) = r^{\ell+1} + a_m r^m$ into Eq. (14), where $a_m$ is assumed to be the next non-zero coefficient in the expansion $(m > \ell + 1)$. We obtain

$$-\frac{\hbar^2}{2\mu}a_m m(m-1)r^{m-2} + V(r)\left(r^{\ell+1} + a_m r^m\right) + \frac{\hbar^2}{2\mu}\ell(\ell+1)\left(a_m r^{m-2}\right) = E(r^{\ell+1} + a_m r^m). \tag{20}$$

The term $a_m r^m$ can be neglected compared to $r^{\ell+1}$. Terms beyond $V_0$ in $V(r)$ are negligible as well. So we have

$$-\frac{\hbar^2}{2\mu}a_m\left[m(m-1) - \ell(\ell+1)\right]r^{m-2} + V_0 r^{\ell+1} = Er^{\ell+1}. \tag{21}$$

Notice that $m(m-1) - \ell(\ell+1) \neq 0$ because $m > \ell+1$. Therefore, we conclude that $m - 2 = \ell + 1$, i.e., the subleading power is

$$m = \ell + 3 = n + 2 \tag{22}$$

and

$$a_m \equiv a_{\ell+3} = \frac{2\mu}{\hbar^2\left[(\ell+3)(\ell+2) - \ell(\ell+1)\right]}(V_0 - E) = \frac{\mu}{(2\ell+3)\hbar^2}(V_0 - E). \tag{23}$$

This also means that $a_{\ell+2} = 0$. We obtain

$$u^E(r) = r^{\ell+1} + \frac{\mu}{(2\ell+3)\hbar^2}(V_0 - E)r^{\ell+3} + ... \tag{24}$$

Notice that $a_{\ell+3}$ depends on the energy $E$. We can thus obtain the short-range behavior of the first energy derivative of $u^E(r)$ (evaluated at $E = 0$)

$$\frac{du^{E=0}(r)}{dE} = -\frac{\mu}{(2\ell+3)\hbar^2} r^{\ell+3} + ... \tag{25}$$

We can see that this is suppressed by $r^2$ compared to the leading-order behavior of $u^E(r)$.

Next, we want to obtain the behavior of the second energy derivative. We can already conclude that it is further suppressed compared to the first energy derivative because only up to linear terms in $E$ appear in the two leading terms of $u^E(r)$ (Eq. (24)). To get the exact behavior we can continue analyzing the expansion. We consider the next term $a_{\ell+4}r^{\ell+4}$ in $u^E(r)$. Substituting it into Eq. (14) gives us as equation involving $r^{\ell+2}$, as lower powers were treated above. We get

$$-\frac{\hbar^2}{2\mu} a_{\ell+4}(\ell+4)(\ell+3) + V_1 + \frac{\hbar^2}{2\mu}\ell(\ell+1)a_{\ell+4} = 0. \tag{26}$$

The energy term on the right-hand-side of Eq. (14) does not contribute because $a_{\ell+2} = 0$, and there is no contribution involving $V_0$ for the same reason. We can isolate $a_{\ell+4}$ and obtain

$$a_{\ell+4} = \frac{\mu}{3(\ell+2)\hbar^2} V_1. \tag{27}$$

This coefficient does not depend on $E$, and therefore does not contribute to energy derivatives. We can continue to the next term, considering $a_{\ell+5}r^{\ell+5}$ in $u^E(r)$. Substituting it into Eq. (14), we obtain an equation involving $r^{\ell+3}$

$$-\frac{\hbar^2}{2\mu}(\ell+5)(\ell+4)a_{\ell+5} + V_0 a_{\ell+3} + V_2 + \frac{\hbar^2}{2\mu}\ell(\ell+1)a_{\ell+5} = E a_{\ell+3}. \tag{28}$$

$a_{\ell+3}$ includes one power of $E$ (Eq. (23)), so $a_{\ell+5}$ includes $E^2$ in its expression coming from the term $E a_{\ell+3}$ above. Explicitly, we get

$$a_{\ell+5} = \frac{\mu}{2(2\ell+5)\hbar^2}\left[(V_0 - E)a_{\ell+3} + V_2\right] = \frac{\mu}{2(2\ell+5)\hbar^2}\left[\frac{\mu}{(2\ell+3)\hbar^2}(V_0 - E)^2 + V_2\right]. \tag{29}$$

Based on the above results, we have

$$u^E(r) = r^{\ell+1} + \frac{\mu}{(2\ell+3)\hbar^2}(V_0 - E)r^{\ell+3} + \frac{\mu}{3(\ell+2)\hbar^2}V_1 r^{\ell+4} + \frac{\mu}{2(2\ell+5)\hbar^2}\left[\frac{\mu}{(2\ell+3)\hbar^2}(V_0 - E)^2 + V_2\right] r^{\ell+5} + ... \tag{30}$$

Therefore, the second energy derivative at short-distances is given by

$$\frac{d^2u^{E=0}(r)}{dE^2} = \frac{\mu^2}{(2\ell+5)(2\ell+3)\hbar^4} r^{\ell+5} + ... \tag{31}$$

This is suppressed by another factor of $r^2$ compared to the first energy derivative. We can also obtain here the subleading term for the first energy derivative.

We can continue to analyze the next orders in the same way, but at this point we can deduce the behavior of all energy derivatives. The first term that includes $E^3$ comes from the $Eu^E(r)$ part of Eq. (14) with the $a_{\ell+5}r^{\ell+5}$ part of $u^E(r)$ (because $a_{\ell+5}$ includes an $E^2$ term). This will be an equation of order $r^{\ell+5}$, which fixes the coefficient $a_{\ell+7}$. So the third energy derivative behaves like $r^{\ell+7}$ at short distances, and each additional energy derivative is suppressed by another factor of $r^2$. Therefore, the $k$-th energy derivative behaves as

$$\frac{d^k u^{E=0}(r)}{dE^k} \propto r^{\ell+1+2k} + ... \tag{32}$$

at short distances. For the wave function $\phi^E(r) \equiv u^E(r)/r$ we obtain

$$\frac{d^k \phi^{E=0}(r)}{dE^k} \propto r^{\ell+2k} + ... \tag{33}$$

This result allows us to organize the different contributions of the short-range expansion presented in the manuscript. The zero-energy $s$-wave function behaves as $\phi_s \sim r^0$ at short distances, so $|\phi_s|^2 \sim 1$, which is the leading order term, that comes with the $C_s^{00}$ contact parameter. Next, the first energy derivative of the $s$-wave solution behaves as $\phi_s^{(1)} \sim r^2$, and the zero-energy $p$-wave solution behaves as $\phi_p^{(0)} \sim r^1$, so both $\phi_s^* \phi_s^{(1)}$ and $|\phi_p|^2$ behave as $r^2$ at short distances. These contributions, therefore, enter together at the next order of the expansion with the contact parameters $C_s^{01}$ and $C_p^{00}$. Next, $\phi_s^{(2)} \sim r^4$, $\phi_p^{(1)} \sim r^3$, and $\phi_d \sim r^2$ ($d$-wave solution) at short distances, so $|\phi_s^{(1)}|^2$, $\phi_s^* \phi_s^{(2)}$, $|\phi_d|^2$ and $\phi_p^* \phi_p^{(1)}$ all behave as $r^4$ and are included at N$^2$LO with the contact parameters $C_s^{11}$, $C_s^{02}$, $C_d^{00}$ and $C_p^{01}$. Next order terms can be similarly identified.

## IV. TWO-BODY FUNCTIONS

In this section we provide more details regarding the two-body wave function $\varphi_\alpha^{(n)}(\boldsymbol{r}_{12})$. As mentioned above, the relevant quantum numbers for nuclear systems are $\alpha = (\pi_\alpha, s_\alpha, j_\alpha, m_\alpha, t_\alpha, t_{z,\alpha})$. In the manuscript, we analyzed neutron matter, so only neutron-neutron ($nn$) pairs are relevant. Therefore, the isospin $t_\alpha$ and isospin projection $t_{z,\alpha}$ are equal to 1 and $-1$, respectively. For realistic nuclear interactions, different values of the orbital angular momentum can be coupled. But, in this work we used a simplified interaction in which any two-body channel has a single orbital angular momentum value $\ell_\alpha$. Due to the Pauli exclusion principle, for $nn$ pairs, $\ell_\alpha + s_\alpha$ must be even. Therefore, positive-parity channels (even $\ell$ values) must have spin $s = 0$, and, thus, $j = \ell$. Specifically, we have a single $s$-wave channel, with $s = 0$ and $j = 0$, and a single $d$-wave channel with $s = 0$ and $j = 2$. Negative-parity channels (odd $\ell$ values) must have spin $s = 1$. Thus, there are in principle 3 different $p$-wave channels as $\ell = 1$ coupled to $s = 1$ can produce $j = 0, 1, 2$. Nevertheless, for the interaction used in our work, the zero-energy two-body functions corresponding to these three channels have exactly the same radial behavior $\phi(r)$. Therefore, they can be considered as a single channel in their contribution to the two-body density and one-body momentum distribution.

We calculate these two-body functions numerically using the Numerov method. For the description of the two-body density it is relevant to look on multiplications of two such functions of the form $\phi_\alpha^{(m)}(r)\phi_\alpha^{(n)}(r)$. This is shown in Fig. 1 including the $s$-wave, $p$-wave, and $d$-wave channels using the AV4' interaction. We can see that the $s$-wave channel with no energy derivatives ($m = n = 0$) is the only contribution which is non-zero at $r = 0$ and is dominant at short-distances. The $s$-wave contribution with $m = 0, n = 1$, and $p$-wave contribution with $m = n = 0$ rise next at somewhat larger distances, providing NLO corrections. The remaining terms shown in the figure are N$^2$LO contributions. We can see that, as claimed in the manuscript, the $s$-wave $m = 0, n = 2$, $s$-wave $m = n = 1$ and $d$-wave $m = n = 0$ terms are very similar, and, therefore, could not be separated in the analysis of the two-body density. We note that also the $p$-wave $m = 0, n = 1$ term has a very similar $r$-dependence, but it comes with spin $s = 1$, while all the others are spin $s = 0$. Since the contacts are fitted to the spin projected two-body densities (see Sec. V), we were able to isolate this $p$-wave contribution.

## V. CONTACT FITTING

As mentioned in the manuscript, we have fitted the contact values to the auxiliary-field diffusion Monte Carlo (AFDMC) calculations of the two-body density. In particular, the spin-projected two-body $nn$ densities $\rho_{nn}^s(r)$ were used for this purpose. As mentioned above, only positive-parity channels contribute to the $s = 0$ $nn$ density, while negative-parity channels contribute to the $s = 1$ $nn$ density. The AFDMC spin-projected $nn$ densities and the result of the fit are shown in Figs. 2 and 3.

[1] R. Weiss, B. Bazak, and N. Barnea, Generalized nuclear contacts and momentum distributions, Phys. Rev. **C92**, 054311 (2015), arXiv:1503.07047 [nucl-th].

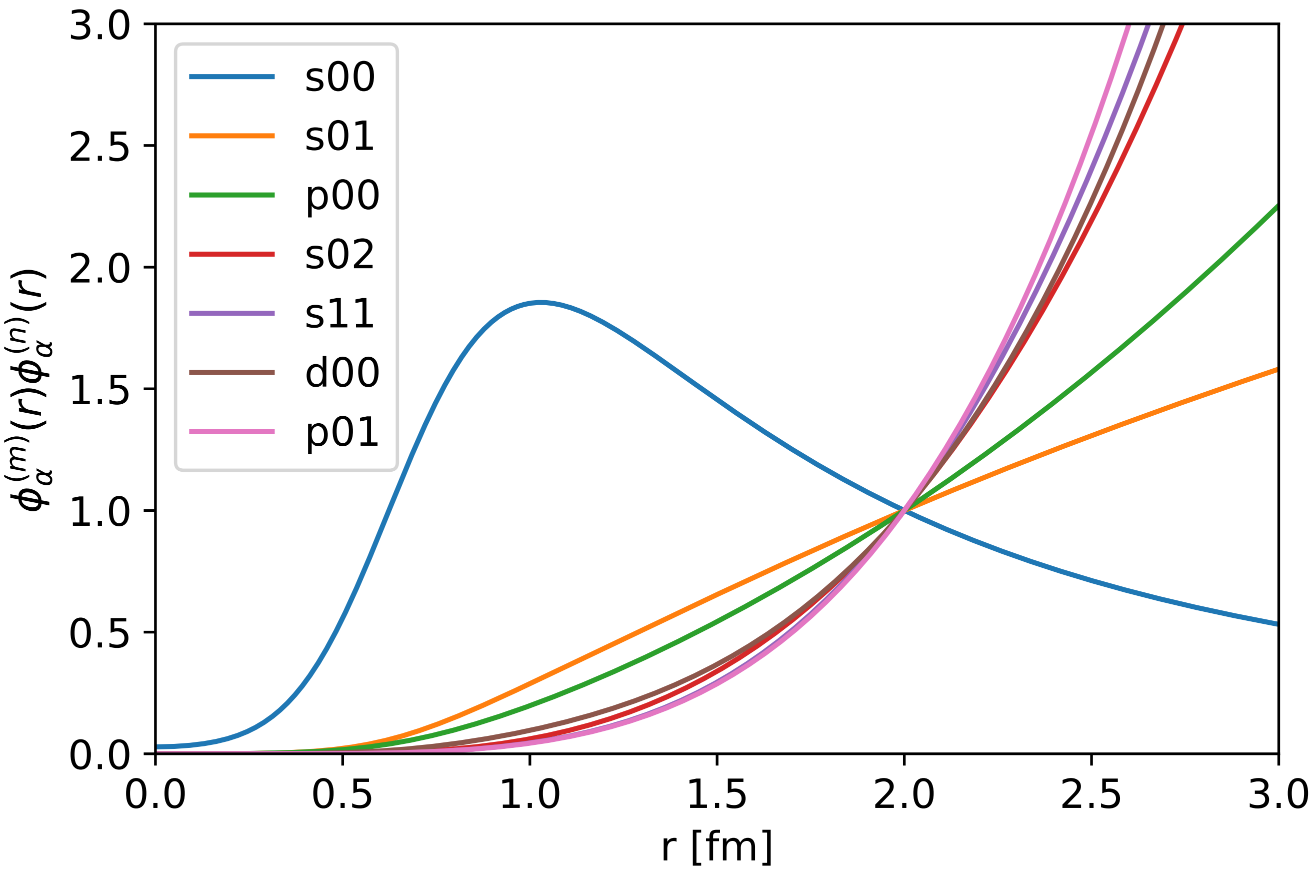


FIG. 1. $\phi_\alpha^{(m)}(r)\phi_\alpha^{(n)}(r)$ functions using the AV4' potential for $nn$ pairs. In the legend, the labels are of the form $\ell_\alpha mn$. $\phi_\alpha^{(n)}(r)$ are normalized to 1 at $r = 2$ fm.

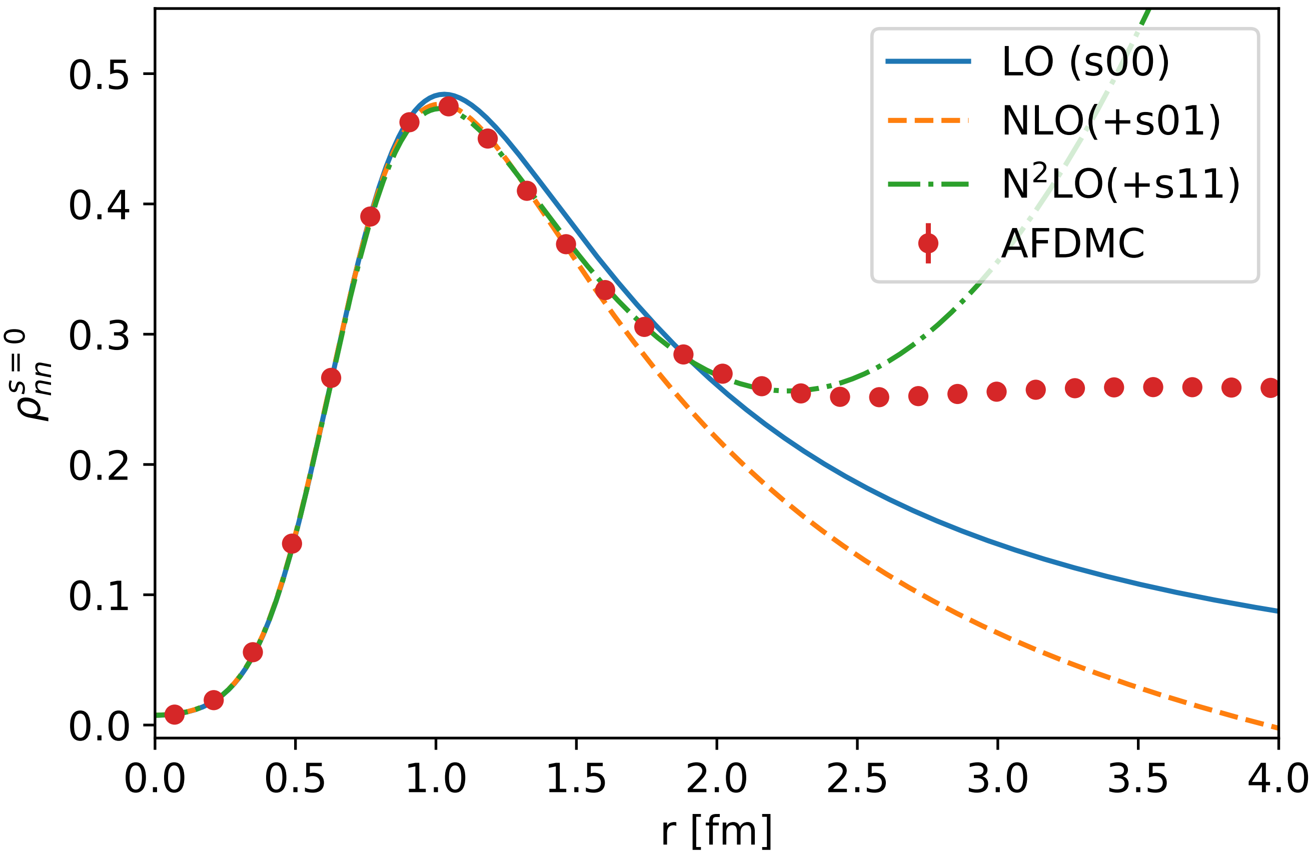


FIG. 2. Fit of the contacts corresponding to positive-parity channels to the spin-zero AFDMC $nn$ density of neutron matter with density of 0.16 fm$^{-3}$. In the legend, the labels are of the form $\ell_\alpha mn$. Since the $s11$, $s02$ and $d00$ cannot be separated, only the the $s11$ term is included at N$^2$LO.

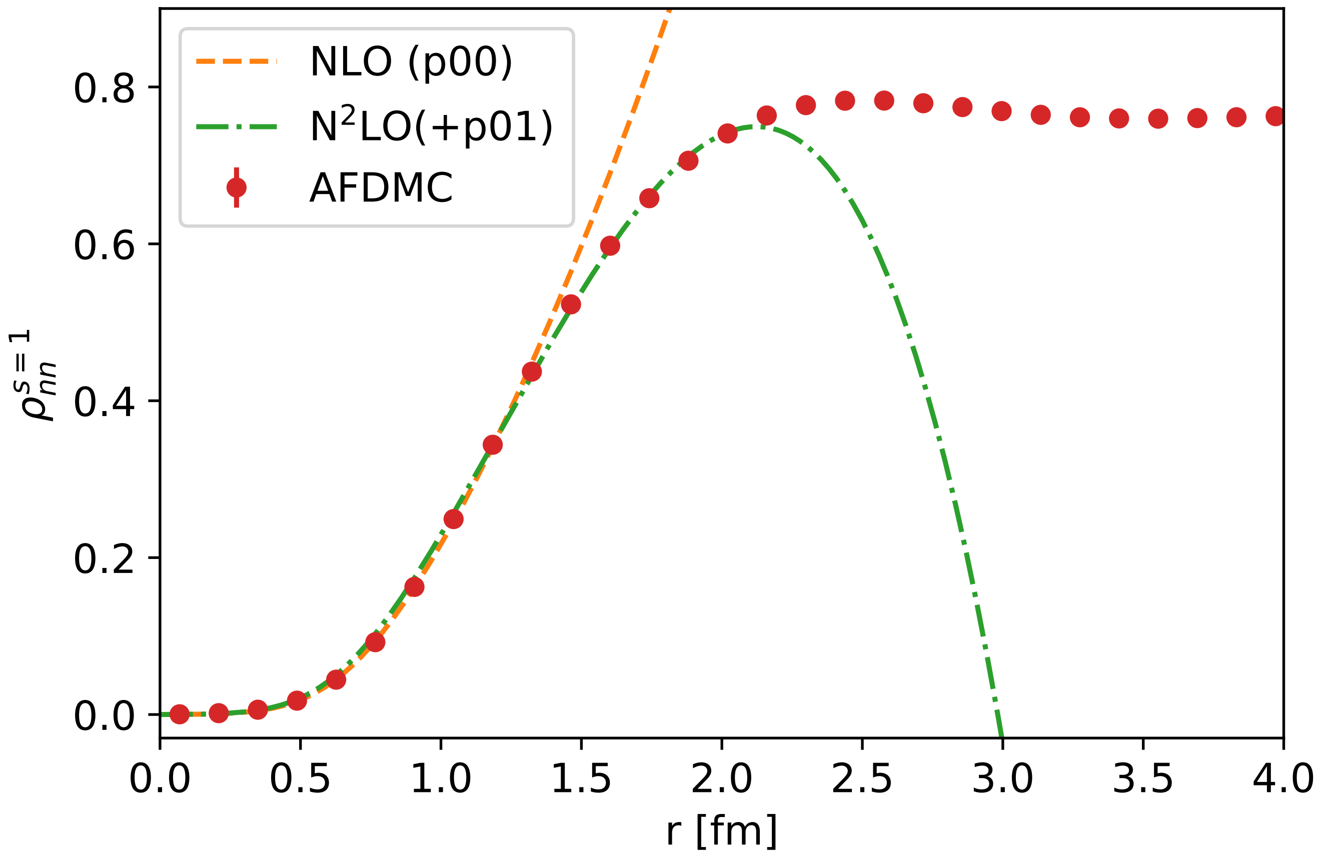


FIG. 3. Fit of the contacts corresponding to negative-parity channels to the spin-one AFDMC $nn$ density of neutron matter with density of 0.16 $\mathrm{fm}^{-3}$. In the legend, the labels are of the form $\ell_\alpha mn$. Notice that there is no LO contribution here because there is no $s$-wave contribution for $nn$ pairs with spin $s = 1$.
